# Supplementary material for: Render In-between: Motion Guided Video Synthesis for Action Interpolation
Source: arXiv:2111.01029 source file (2021-11-01)
Supplement: Supplementary file 1 [file 0327_supp_arxiv.pdf]

# Supplementary Material for
# "Render In-between: Motion Guided Video Synthesis for Action Interpolation"

Hsuan-I Ho[1] Xu Chen[1,2] Jie Song[1] Otmar Hilliges[1]
[1]Department of Computer Science, ETH Zürich
[2]Max Planck Institute for Intelligent Systems, Tübingen

**Summary.** In Sec. A, we provide more information about our proposed dataset. In Sec. B, we detail the design of our human motion modelling networks and the pose-guided neural rendering model, including the architecture, the training scheme and the hyper-parameters. In Sec. C, we show additional qualitative results in comparison with baseline methods for human motion modelling, human image generation and video interpolation.

## A. HumanSloMo Dataset

In this section, we provide more details about the dataset of videos of human activities **HumanSloMo**. We collect high-quality, high frame-rate videos from YouTube and also adopt the standard frame-rate videos provided in [2]. In total, the dataset contains 5 different activity categories with 80 action clips performed by 10 subjects in total. Table A summarizes the videos of 5 categories alongside other dataset properties. Examples of video thumbnails can be found at Fig. J. We downsample the video frames to 15 FPS for test, from which high FPS sequences are to be recovered.

| **Category** | **Resolution** | **(a)** | **(b)** | **(c)** |
|---|---|---|---|---|
| Dance [2] | 1024x512 | 10 | 878 | 82 |
| Body Training | 1920x1080 | 15 | 798 | 78 |
| Boxing | 1920x1080 | 15 | 1394 | 121 |
| Basketball | 1920x1080 | 13 | 368 | 35 |
| Martial Arts | 1920x1080 | 27 | 1054 | 142 |

Table A: **Details about HumanSlomo dataset**. Note that (a) is the number of clips for the video category, (b) denotes the number of low FPS frames for training, (c) lists the numbers of triplets (3-frame sequences) used for evaluation.

## B. Implementation Details

### B.1. Human Motion Modeling

We adopt the transformer architecture in [1] as the backbone for our human motion modelling networks. An attention layer converts input features into three representations: *query*, *key*, and *value*. If the *query* and the *key* are highly correlated (with higher value from dot-product), its *value* is considered relevant to the *query* correspondingly. Hence, the final results are yielded from multiplying the softmax of attention weights and values. To achieve human motion modelling in our denoising network and interpolation network, we uniquely employ attention masks to control where and when to attend the necessary poses across time steps.

The detailed architecture of both motion denoising network and motion interpolation network is illustrated in Fig. A. For both networks, we use $N = 6$ attention blocks. We set the number of heads in the attention layer to be $M = 8$, the dropout probability to be $0.1$ and use leaky ReLU as the activation function.

We use 13437 motion sequences from the AMASS dataset for training and 504 sequences for validation. When generating 2D joints, we randomly apply perturbation, joints dropping and flipping to $15\% \sim 25\%$ joints to simulate the noises and errors in actual pose detections. We train our network using Adam optimizer with an initial learning rate of $10^{-4}$, a batch size of

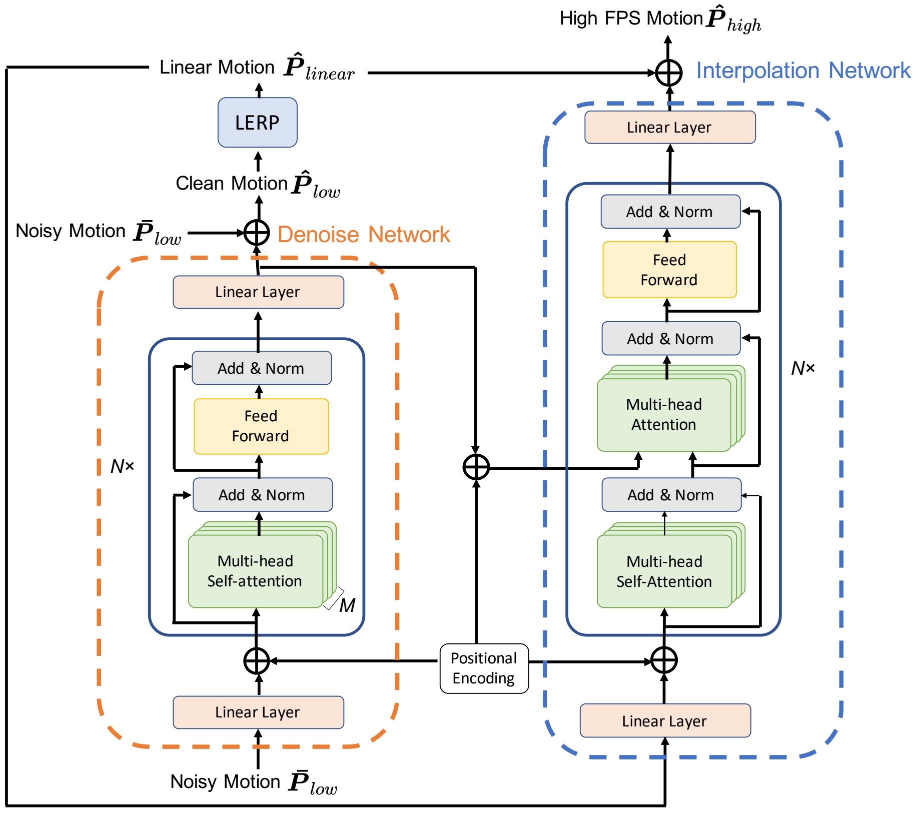


Figure A: **Detailed Network architecture of the human motion modeling network.** We implement our network based on the transformer in [1] using PyTorch. For both networks, we use $N = 6$ attention blocks. We set the number of heads in the attention layer to be $M = 8$, the dropout probability to be 0.1 and use leaky ReLU as activation function.

32, and first- and second-momentum of 0.5 and 0.99 respectively. The learning rate is decayed with a scale of 0.5 for every 100 epochs. We set the weight of the interpolation loss $\lambda_{interp} = 2$. The training takes one day on a RTX 2080Ti for 300 epochs.

## B.2. Human Image Generation Network

Fig. B depicts the detailed architecture of our neural rendering model. Our model is adapted from [5] which consists an encoder-decoder based network $G_s$ with SPADE residual blocks (Fig. C) and a conditional feature encoder $E_c$. The conditional features are extracted and fed into the SPADE residual blocks for providing pose-aware appearance information. The SPADE residual network would try to recover human images according to the input poses with the assistance of conditional features. To further take the background dynamics and consistency into consideration, a mask generator $G_m$ predicts alpha blending masks to composite generated foreground bodies with background images. Finally, a patchGAN [3] based image discriminator $D$ is deployed to ensure the generator would produce perceptually realistic images. We further train two separated discriminators for the cropped area of human face and fists. Table. B lists detailed components used in our model.

Besides the loss described in Sect. 3.3, the LSGAN [4] loss is applied to the neural rendering model and the discriminator during training. The adversarial loss applied to the discriminator is formulated as:

$$\begin{aligned}\mathcal{L}_{adv}^{D} = \frac{1}{2}\mathbb{E}_{(\boldsymbol{p}_t,\hat{I}_t)}\left[D(\boldsymbol{p}_t,\hat{I}_t)^2\right] + \\ \frac{1}{2}\mathbb{E}_{(\boldsymbol{p}_t,I_t)}\left[(D(\boldsymbol{p}_t,I_t)-1)^2\right].\end{aligned} \tag{A}$$

The adversarial loss for generator is calculated as:

$$\mathcal{L}_{adv}^{G} = \mathbb{E}_{(\boldsymbol{p}_t,\hat{I}_t)}\left[\left(D(\boldsymbol{p}_t,\hat{I}_t)-1\right)^2\right] + \lambda_{FM}\mathcal{L}_{FM}, \tag{B}$$

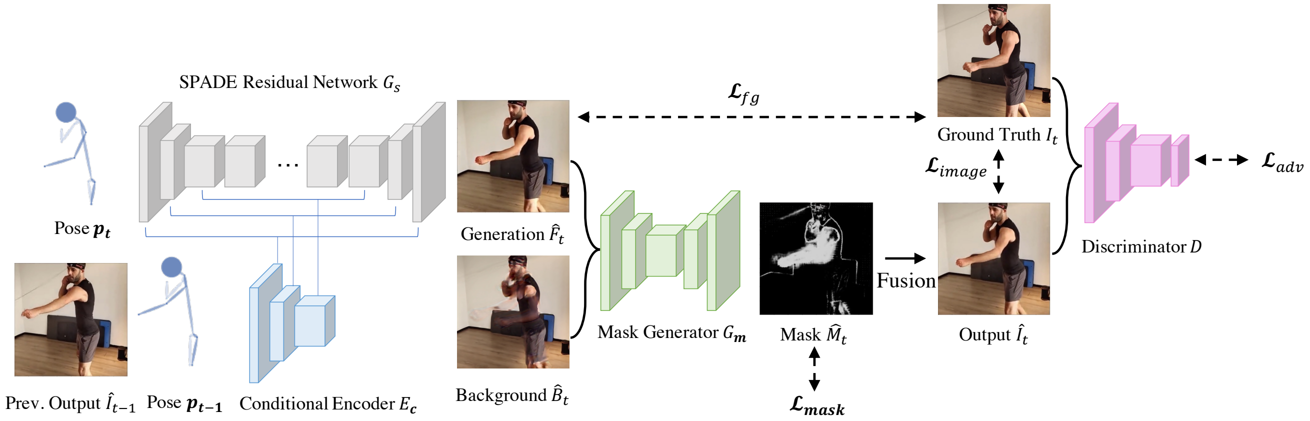


Figure B: **Network architecture of our human image generation network.** Our model is modified from [5] which consists an encoder-decoder based network $G_s$ with SPADE residual blocks (Fig. C) and a conditional feature encoder $E_c$. An additional mask generator $G_m$ learns to composite the generated foreground image with the input background image. Finally, a PatchGAN [3] based image discriminator is deployed to ensure the generator produce perceptually realistic images.

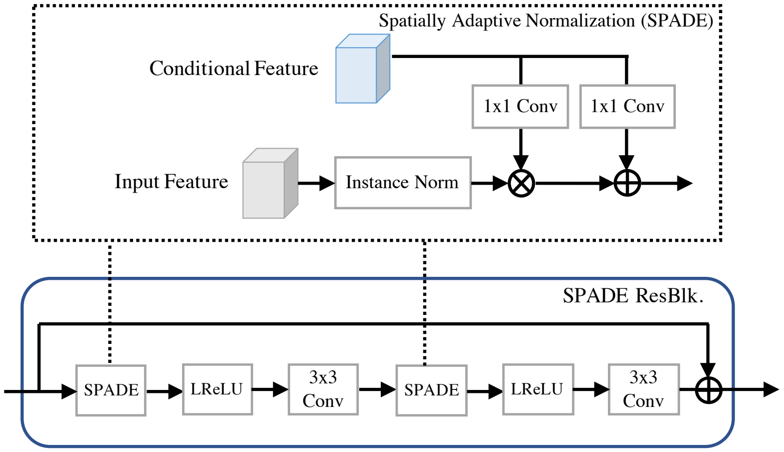


Figure C: **Components of SPADE residual block.** The SPADE residual block contains two spatially adaptive normalization (SPADE) layers, two leaky ReLU layers, and two convolutional layers. The conditional feature provides additional pose-aware appearance information for generating the human body via spatially adaptive normalization.

where the discriminator's feature-matching loss $\mathcal{L}_{FM}$, comparing the real and generated image using the activations of the discriminator, is calculated as:

$$\mathcal{L}_{FM} = \mathbb{E}_{(\boldsymbol{p}_t, I_t, \hat{I}_t)} \sum_{j=1}^{M} \frac{1}{N_j} \| D^{(j)}(\boldsymbol{p}_t, \hat{I}_t) - D^{(j)}(\boldsymbol{p}_t, I_t) \|_1. \tag{C}$$

With $M$ being the number of discriminator layers, $N_j$ the number of elements in the j-th layer. The expectation is computed per mini-batch, over the input $\boldsymbol{p}_t$, $I_t$, and $\hat{I}_t$.

We train our network using Adam optimizer with a learning rate of $10^{-4}$ for the neural rendering network, $4 \times 10^{-4}$ for the discriminator, and first- and second-momentum of 0 and 0.99. For each training iteration, we sample $K = 3$ continuous frames as a training sample and recovery the middle frames in each feed-forward pass. Random cropping and rotation are applied to the training images for data augmentation. To mitigate possible overfitting to the input background images, we also blur out random human body parts in background images. The batch size is set to 2, $K$ is increased by 1 and the learning rate is decayed with a scale of 0.5 for every 12 epochs. We set the weights of the loss terms to be $\lambda_{FM} = 10$, $\lambda_{percep} = 0.5$, $\lambda_{im} = 10$, $\lambda_{fg} = 10$, $\lambda_{mask} = 2.0$ across all experiments. The training takes one day on a RTX 2080Ti for 60 epochs.

| | layer type(s) | out channels | stride | activation |
|---|---|---|---|---|
| SPADE Residual Network | | | | |
| 1 | 3×3 Conv | 16 | 1 | LReLU |
| 2 | 3×3 SPADE ResBlk. | 32 | 1 | LReLU |
| | 3×3 Avg. Pooling | | 2 | |
| 3 | 3×3 SPADE ResBlk. | 64 | 1 | LReLU |
| | 3×3 Avg. Pooling | | 2 | |
| 4 | 3×3 SPADE ResBlk. | 128 | 1 | LReLU |
| | 3×3 Avg. Pooling | | 2 | |
| 5 | 3×3 SPADE ResBlk. | 256 | 1 | LReLU |
| | 3×3 Avg. Pooling | | 2 | |
| 6 | 3×3 SPADE ResBlk. × 6 | 512 | 1 | LReLU |
| 7 | 3×3 SPADE ResBlk. | 256 | 1 | LReLU |
| | UpSampling | | 2 | |
| 8 | 3×3 SPADE ResBlk. | 128 | 1 | LReLU |
| | UpSampling | | 2 | |
| 9 | 3×3 SPADE ResBlk. | 64 | 1 | LReLU |
| | UpSampling | | 2 | |
| 10 | 3×3 SPADE ResBlk. | 32 | 1 | LReLU |
| | UpSampling | | 2 | |
| 11 | 3×3 SPADE ResBlk. | 16 | 1 | LReLU |
| 12 | 1×1 Conv | 3 | 1 | Tanh |
| Conditional Feature Encoder | | | | |
| 1 | 3×3 Conv | 64 | 1 | LReLU |
| 2 | 3×3 Conv | 128 | 2 | LReLU |
| 3 | 3×3 Conv | 256 | 2 | LReLU |
| 4 | 3×3 Conv | 512 | 2 | LReLU |
| 5 | 3×3 Conv | 1024 | 2 | LReLU |
| Mask Generator | | | | |
| 1 | 3×3 Conv, IN | 32 | 1 | LReLU |
| 2 | 3×3 Conv, IN | 64 | 2 | LReLU |
| 3 | 3×3 Conv, IN | 128 | 2 | LReLU |
| 4 | 3×3 Conv, IN | 256 | 2 | LReLU |
| 5 | 3×3 Conv, IN × 4 | 256 | 1 | LReLU |
| 6 | 3×3 ConvT, IN | 128 | 2 | LReLU |
| 7 | 3×3 ConvT, IN | 64 | 2 | LReLU |
| 8 | 3×3 ConvT, IN | 32 | 2 | LReLU |
| 9 | 1×1 ConvT | 1 | 1 | Sigmoid |
| Discriminator | | | | |
| 1 | 3×3 Conv, IN | 32 | 1 | LReLU |
| 2 | 3×3 Conv, IN | 64 | 2 | LReLU |
| 3 | 3×3 Conv, IN | 128 | 2 | LReLU |
| 4 | 3×3 Conv, IN | 256 | 2 | LReLU |
| 5 | 3×3 Conv, IN | 512 | 2 | LReLU |
| 6 | 1×1 Conv | 1 | 1 | Sigmoid |

Table B: **Network details of the neural rendering model.** ‘LReLU’ denotes leaky ReLU activation, and ’IN’ denotes instance normalization layer, and ’ConvT’ denotes transposed convolution layer.

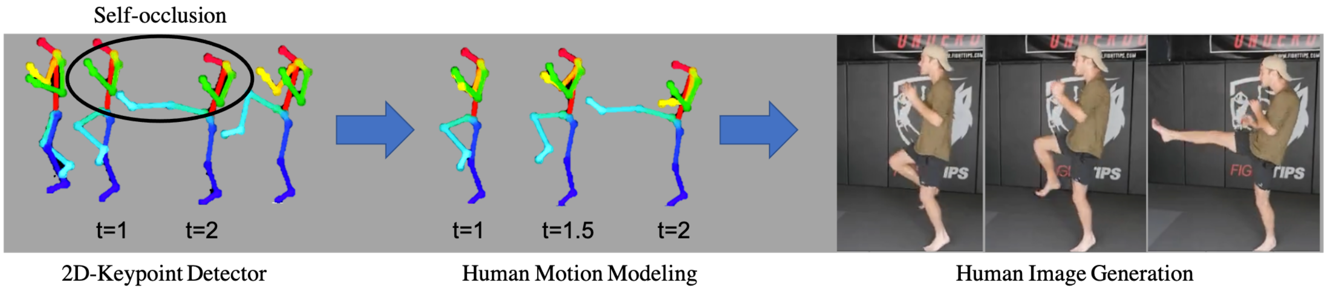


Figure D: **Example of body occlusion.** Even a part of human body is occluded, the motion modelling network can still generate accurate motion for the visible parts and hallucinate the occluded parts. Our neural rendering model can use the previous generated frames and the providing pose to generate plausible human images.

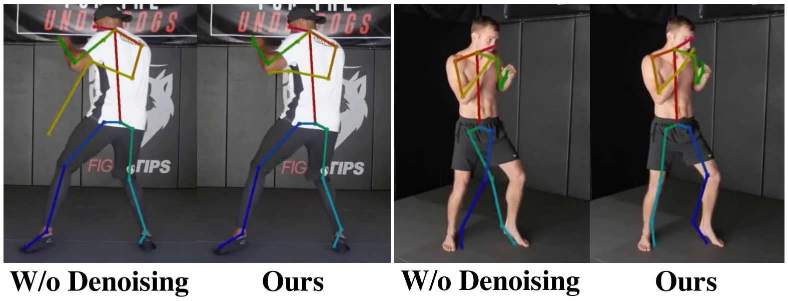


Figure E: **Visualization of interpolated poses.** We overly the predicted poses on the ground-truth images. Our method is robust to noisy detections and produces more realistic pose.

| | No occlusion | 20% occlusion |
|---|---|---|
| Ours | 0.456 | 0.668 (-45.6%) |
| W/o denoising | 0.474 | 1.980 (**-317.7%**) |

Table C: **Analysis of joint occlusion**. We report average L1 loss on our full model and the variant of training without noisy/missing joints. Without our training strategy, occlusion can introduce 3 times more error to motion modelling.

# C. Additional Results

## C.1. Robustness to Joint Occlusion and Error

We provide additional details and experiments to explain how our human motion model tackles with joint occlusion. Since our model is trained with noise and randomly drop-out joints, it learns to infer occluded joints from the nearby joints positions and temporal patterns. As shown in Fig. D, in a case where a proportion of body joints are consistently occluded, the motion modelling network can still generate accurate motion for the visible parts and hallucinate the occluded parts. While the hallucination might not agree with the ground-truth motion, the neural rendering model can still use the previous generated frames and the providing pose to generate plausible human images. To further quantify this, we simulate occlusions by randomly removing 20% joints in 20% of the test motion sequences. Without our training strategy, the avg L1 error increases from 0.668 to 1.980. This corresponds to a *317.7%* error increase over the full joint condition (0.474) whereas ours is only impacted by *46.5%* (see Table C).

Fig. F visualize the ablation study in Sect. 4.3 and the effect of our training strategy. It can be seen that false and missing input joints can largely influence the resulting motion. Fig. E shows a practical example that our motion model is able to correct the false detections from off-the-shelf 2D pose detectors. If the model is trained without denoising function (i.e., simply follow the linearly interpolated motion), the false skeletal images could influence the later generation of human bodies.

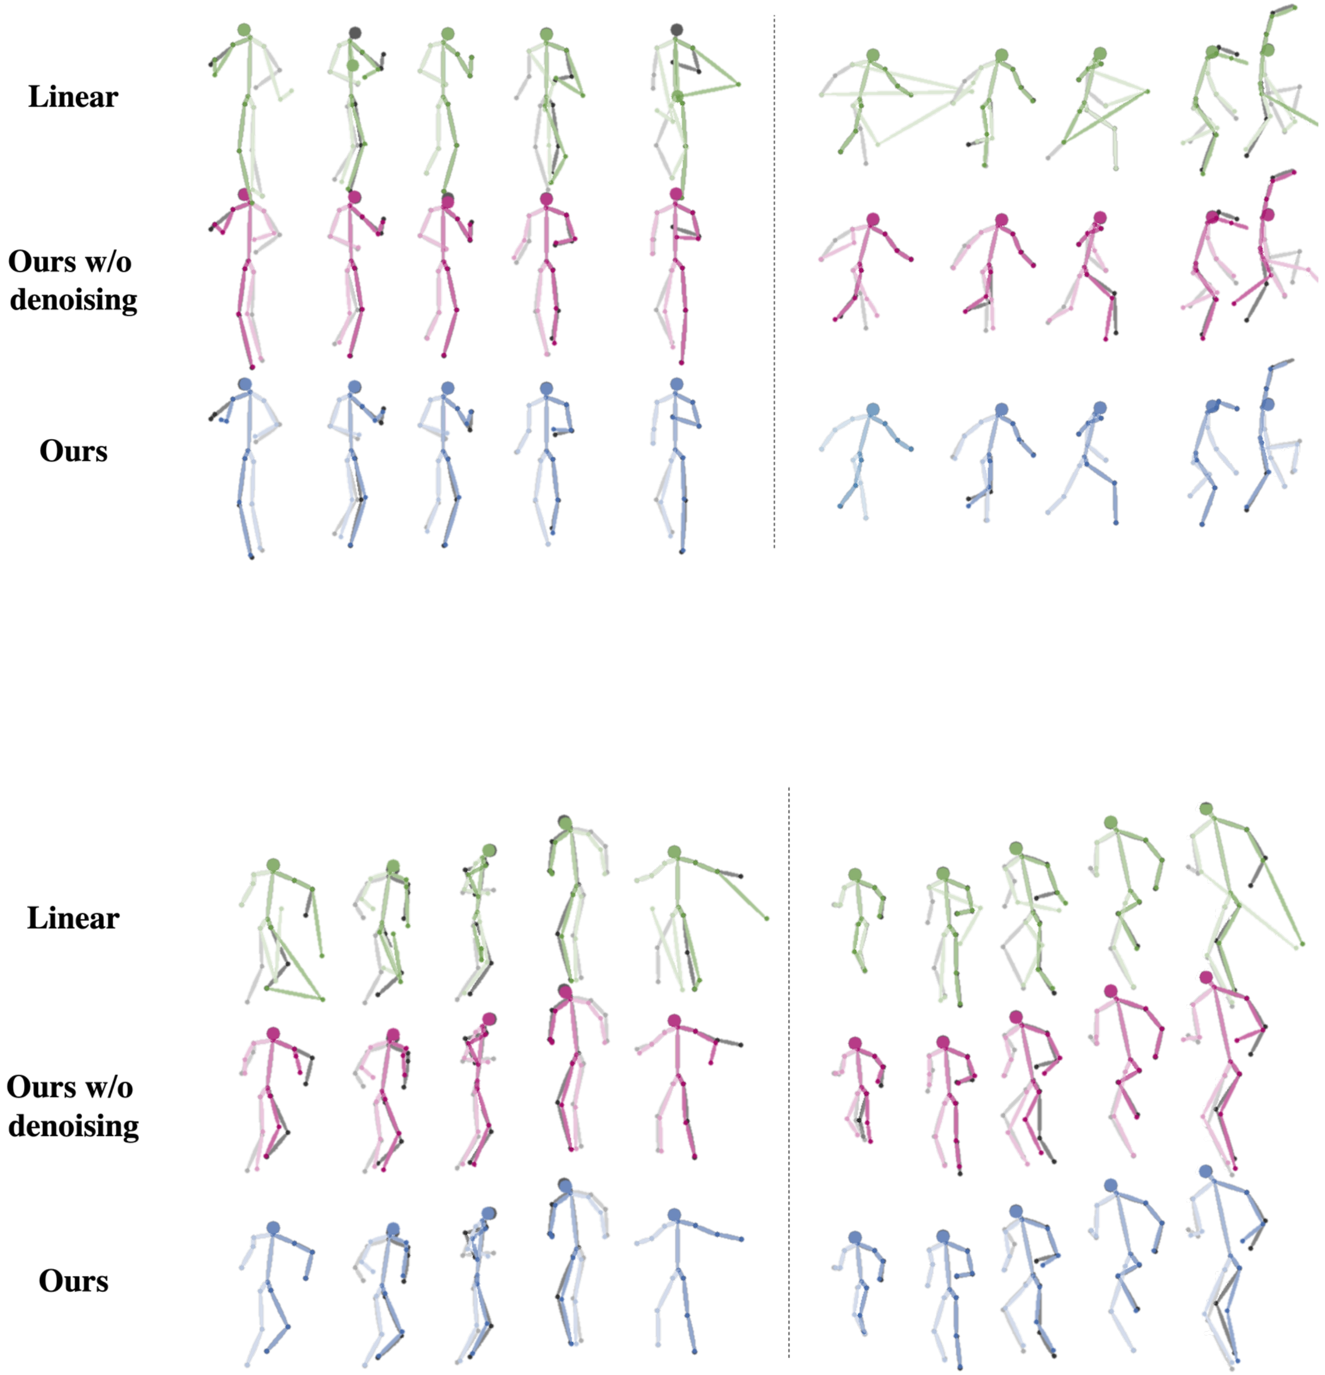


Figure F: **Qualitative results of human motion modelling on AMASS**. We overly the results from our method *(blue)*, our method without the denoising network *(red)*, and linear interpolation *(green)* with the ground truth *(gray)*. Our generated motion is closer to the ground-truth, and contains less erroneous joints.

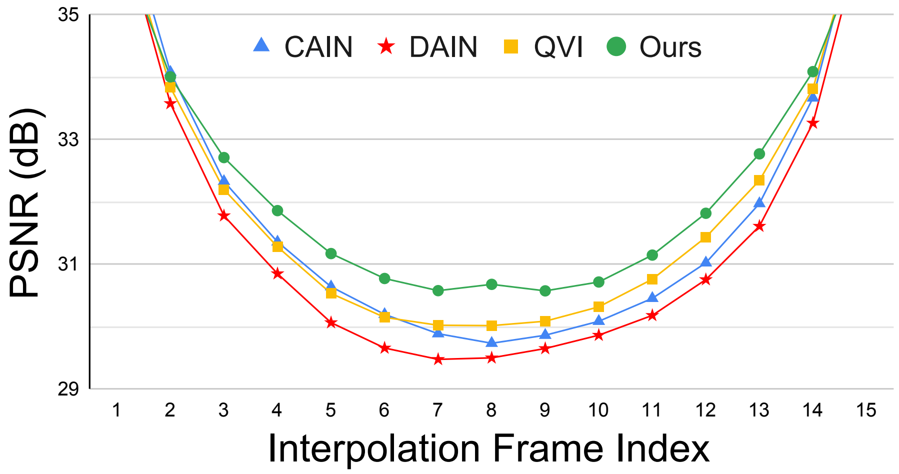


Figure G: **Performance stability over time.** We generate 15 frames between two existing frames 0 and 16 using our method and three state-of-the-art baselines CAIN, DAIN and QVI. Our method performs consistently well over time and can better handle frames far away from the input low FPS frames.

### C.2. Performance Stability for Multi-frame Interpolation.

Intuitively, the quality of interpolated frames depends on the distance to the sources in time horizon. In contrast to the evaluation protocol defined in Sec. 4.1 where only one frame is generated between two consecutive frames, 15 frames are generated between two low FPS video frames (indexed as 0 and 16) by our method and the other three best performing baselines, namely **CAIN**, **DAIN** and **QVI**. As shown in Fig. G, existing methods have small error near input frames, but larger error when interpolated frames are far away from input ones, e.g. frame 8. On the other hand, since our method generates images conditioned on the pose produced by motion model, the generation quality is more consistent along the interpolated frame index.

### C.3. Additional Qualitative Comparisons

Fig. H shows the qualitative comparison between our method and existing human image generation networks. We train their network [6, 7] using the same data as ours (i.e., the low FPS videos). Since these methods do not consider human pose interpolation, we provide them ground-truth pose as input for inference. As can be seen, our method can better handle background dynamic and human appearance details such as background shadow and body texture.

We provide more qualitative comparisons with SOTA video interpolation methods on the test sequences of HumanSlomo in Fig. J. On the other hand, Fig. I shows some failure cases of our method. The neural rendering module might produce artifacts if the background and foreground share similar texture. It might also generate body parts that lose 3D details since 2D skeletons cannot capture the 3D body structure well. We believe this is an interesting direction for future work, for example modelling the human motion and generating human bodies with more complex 3D body representations.

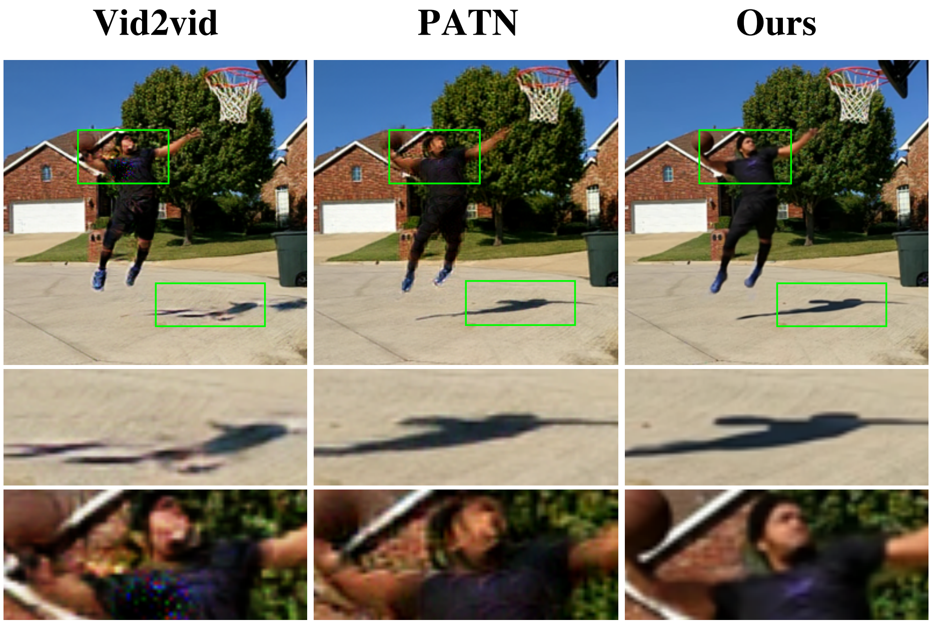


Figure H: **Qualitative comparison with state-of-the-art human image generation methods.** We show that the direct use of their methods would not produce desirable image details such as background shadow and body texture.

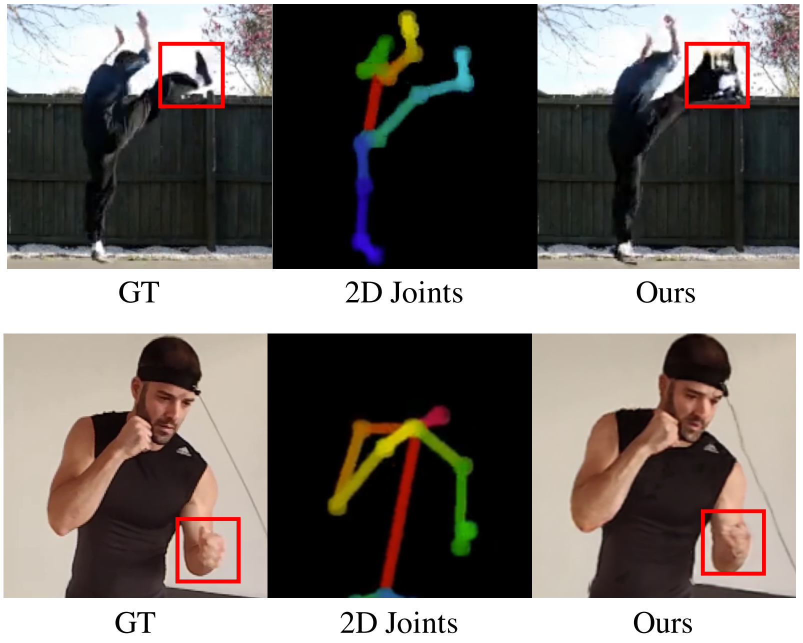


Figure I: **Failure cases.** *Top:* A case that failed to generate correct body textures. *Bottom:* A failure case that lose 3D structural details due to the limitation of 2D skeleton.

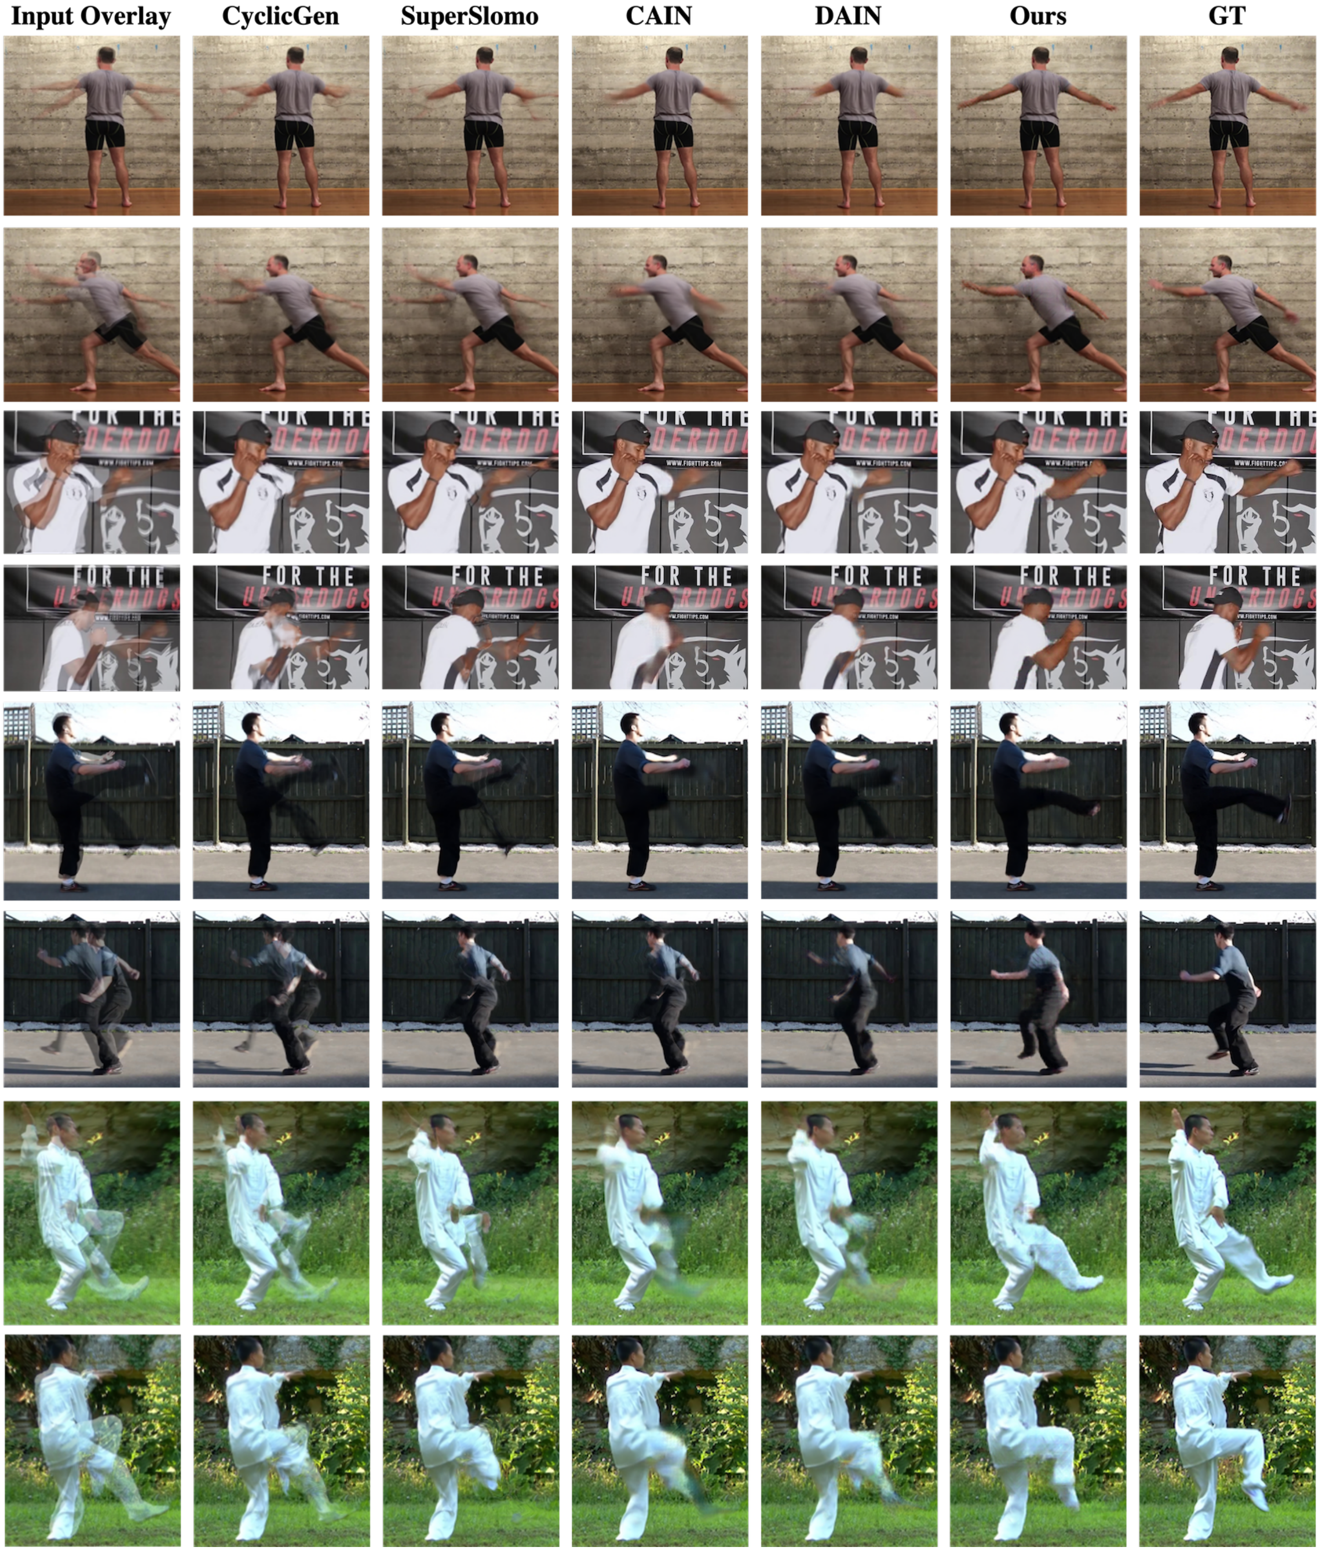
Input Overlay
CyclicGen
SuperSlomo
CAIN
DAIN
Ours
GT

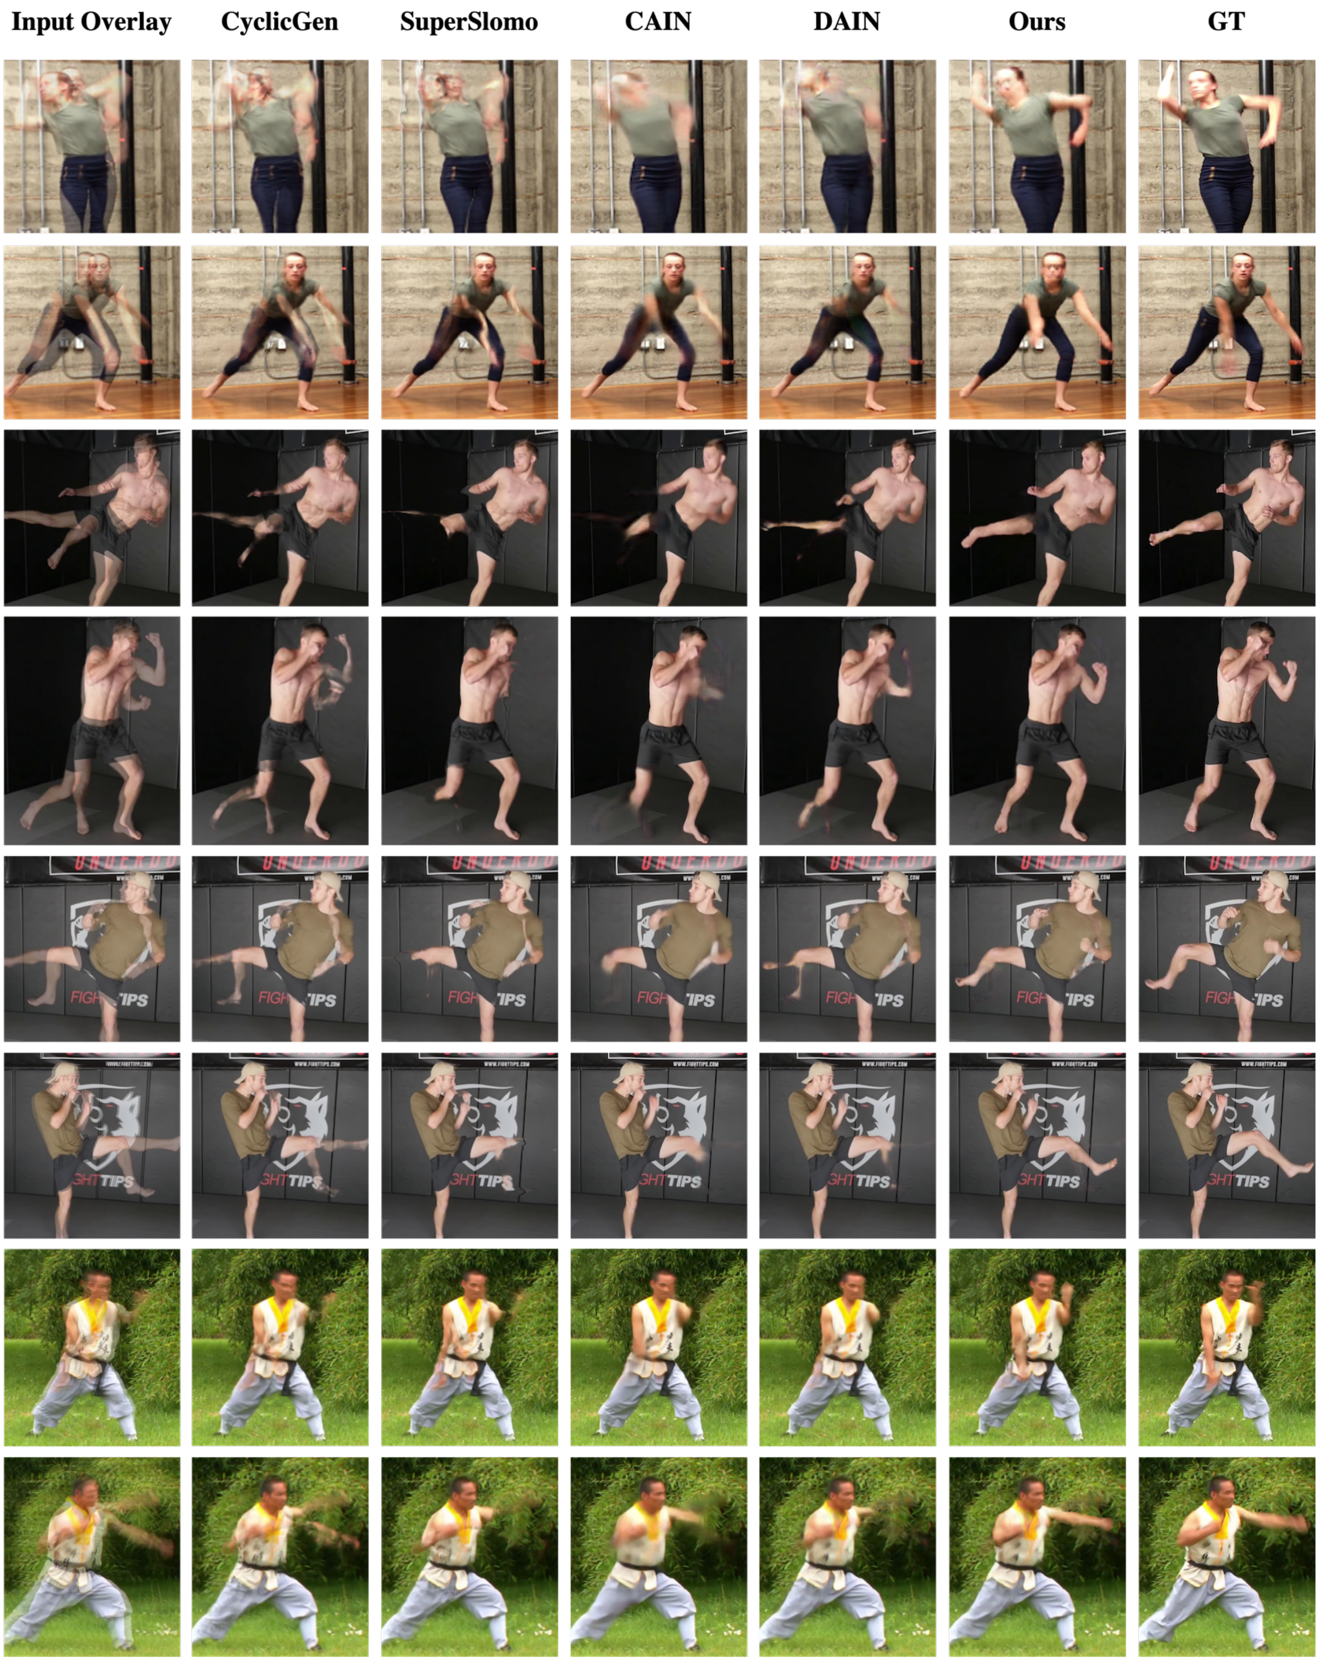


Figure J: **Additional qualitative results on HumanSloMo dataset.**

## References


[1] Nicolas Carion, Francisco Massa, Gabriel Synnaeve, Nicolas Usunier, Alexander Kirillov, and Sergey Zagoruyko. End-to-end object detection with transformers. *arXiv preprint arXiv:2005.12872*, 2020. 1, 2

[2] Caroline Chan, Shiry Ginosar, Tinghui Zhou, and Alexei A Efros. Everybody dance now. In *Proceedings of the IEEE International Conference on Computer Vision (ICCV)*, 2019. 1

[3] Phillip Isola, Jun-Yan Zhu, Tinghui Zhou, and Alexei A Efros. Image-to-image translation with conditional adversarial networks. In *Proceedings of the IEEE Conference on Computer Vision and Pattern Recognition (CVPR)*, 2017. 2, 3

[4] Xudong Mao, Qing Li, Haoran Xie, Raymond YK Lau, Zhen Wang, and Stephen Paul Smolley. Least squares generative adversarial networks. In *Proceedings of the IEEE International Conference on Computer Vision (ICCV)*, 2017. 2

[5] Taesung Park, Ming-Yu Liu, Ting-Chun Wang, and Jun-Yan Zhu. Semantic image synthesis with spatially-adaptive normalization. In *Proceedings of the IEEE Conference on Computer Vision and Pattern Recognition (CVPR)*, 2019. 2, 3

[6] Ting-Chun Wang, Ming-Yu Liu, Jun-Yan Zhu, Guilin Liu, Andrew Tao, Jan Kautz, and Bryan Catanzaro. Video-to-video synthesis. In *Advances in Neural Information Processing Systems (NIPS)*, 2018. 7

[7] Zhen Zhu, Tengteng Huang, Baoguang Shi, Miao Yu, Bofei Wang, and Xiang Bai. Progressive pose attention transfer for person image generation. In *Proceedings of the IEEE Conference on Computer Vision and Pattern Recognition (CVPR)*, 2019. 7
